# Supplementary material for: Complexity Estimates for Fourier-Motzkin Elimination
Source: arXiv:1811.01510 source file (2019-05-10)
Supplement: Supplementary file 1 [file Appendix.tex]

\section{Proofs} %% Appendix A
\label{ap:proofs}

\subsection{Proof of Lemma \ref{le:projcharcone}} %% Appendix
%% A.1
\label{ap:projcharcone}
\input{projection_charcone_commute_proof}

\subsection{Proof of Theorem \ref{thm:polarcone}} %% Appendix A.2
\label{ap:polarcone}
\input{polarcone_theorem_proof.tex}

\subsection{Proof of Lemma \ref{le:initialprojection}}
\label{ap:initialprojection}
\input{initial_projection_proof}

\subsection{Proof of Lemma \ref{le:extcoefbound}} %% Appendix A.3
\label{ap:extcoefbound}
\input{extreme_ray_bound}

\subsection{Proof of Lemma \ref{le:ddcomp}} %% Appendix A.4
\label{ap:ddcomp}
\input{dd_complexity}

\subsection{Proof of Lemma \ref{le:compcrtc}} %% Appendix A.5
\label{ap:compcrtc}
\input{detailed_comp}

\subsection{Proof of Lemma \ref{le:extremeraycheck}} %% Appendix A.6
\label{ap:extremeraycheck}
\input{check_extreme_ray_proof}

\subsection{Subsumption cone}
\label{ap:subsumptionProof}
\input{subsumption_cone_proof}

\section{Double description method} %% Appendix B
\label{ap:ddmethod}
\input{DDmethod_algorithm}
